# Supplementary material for: Estimating Uncertainty of Omnimodal Large Language Models via External Omnimodal Embeddings
Source: arXiv:2610.16933 source file (2026-10-12)
Supplement: Supplementary file 1 [file artifact_description.tex]

\section{Artifact Documentation.}
Our experiments use UNO-Bench, a unified benchmark for evaluating omni-modal large language models across both uni-modal and omni-modal understanding capabilities. UNO-Bench comprises 44 task types spanning perception and reasoning abilities under a unified capability taxonomy, covering image, video, audio, and text modalities as well as their combinations. The benchmark contains 1,250 human-curated omni-modal samples and 2,480 enhanced uni-modal samples, with the omni-modal portion designed such that approximately 98\% of the questions require information from multiple modalities for successful resolution.

UNO-Bench includes both multiple-choice and multi-step open-ended questions, enabling the evaluation of perception, cross-modal alignment, temporal reasoning, spatial reasoning, and complex multi-step reasoning. The benchmark covers diverse application domains, including everyday scenarios, society, culture, art, science, mathematics, document understanding, and audiovisual reasoning, using real-world images, videos, and human-recorded audio.

The benchmark contains both English and Chinese data. In particular, the manually curated omni-modal dataset was designed to better reflect real-world scenarios in Chinese linguistic contexts while also including English-language content. Human annotators, including domain experts and crowd workers, constructed the benchmark through a human-centric annotation pipeline with multiple rounds of model-assisted and manual quality control.

UNO-Bench was not specifically designed for fairness or demographic evaluation. Although the collected multimedia content includes people from a variety of real-world contexts, the benchmark does not provide demographic annotations or guarantee balanced representation across demographic groups. Consequently, our evaluation does not support conclusions regarding fairness or subgroup performance.

As UNO-Bench is a benchmark for evaluating multimodal understanding rather than demographic characteristics, any biases present in the underlying media, annotations, or cultural contexts may be reflected in model performance. We therefore interpret our uncertainty estimation results as measurements of model calibration on the benchmark tasks rather than indicators of fairness or general societal performance.
