# Supplementary material for: Estimating Uncertainty of Omnimodal Large Language Models via External Omnimodal Embeddings
Source: arXiv:2610.16933 source file (2026-10-12)
Supplement: Supplementary file 2 [file sampling_free.tex]

\section{The Strictly Single-Generation Regime}
\label{app:single-chain}
\label{sec:single-chain}

The main protocol scores a fixed, majority-selected answer and, for the embedding-based methods, forms the confidence by aggregating per-chain scores over the candidate pool (the sum-share of Section~\ref{sec:experimental-setup}). The cheapest conceivable deployment instead produces \emph{exactly one} chain and scores it in isolation; this appendix evaluates that regime directly. Each question is represented by its first sampled generation (all candidates are exchangeable draws at temperature 1.0), scored by its own per-chain value, with that generation's own correctness as the label; no clustering or aggregation of any kind is used. $\mathcal{C}_{\text{chain}}$ is refitted on the canonical partition's validation items under the published protocol, with model selection likewise performed single-chain. Table~\ref{tab:single-chain} reports the results (ECE is omitted: in this regime it is governed by the same scale artefacts analysed in Appendix~\ref{app:variance}, and Platt calibration applies unchanged).

\begin{table*}[t]
\centering
\begin{adjustbox}{width=\textwidth}
\begin{tabular}{l cc cc cc cc cc}
\toprule
& \multicolumn{2}{c}{Avg} & \multicolumn{2}{c}{Audio} & \multicolumn{2}{c}{MC} & \multicolumn{2}{c}{MO} & \multicolumn{2}{c}{Visual} \\
\cmidrule(lr){2-3} \cmidrule(lr){4-5} \cmidrule(lr){6-7} \cmidrule(lr){8-9} \cmidrule(lr){10-11}
Method & AUROC & AURAC & AUROC & AURAC & AUROC & AURAC & AUROC & AURAC & AUROC & AURAC \\
\midrule
Level-Based Conf. & 0.557 & 0.670 & 0.540 & 0.843 & 0.531 & 0.602 & 0.583 & 0.411 & 0.573 & 0.823 \\
Self-Probing Conf. & \textbf{0.629} & \textbf{0.715} & 0.610 & 0.857 & \textbf{0.590} & \textbf{0.666} & \textbf{0.671} & 0.483 & \textbf{0.643} & \textbf{0.852} \\
Two-Step CoT Conf. & 0.608 & 0.707 & 0.600 & 0.862 & 0.568 & 0.624 & 0.663 & \textbf{0.499} & 0.602 & 0.841 \\
\midrule
$S_{\text{smooth}}$ & 0.476 & 0.629 & 0.521 & 0.823 & 0.497 & 0.596 & 0.392 & 0.348 & 0.494 & 0.750 \\
$S_{\text{dens}}$ & 0.471 & 0.621 & 0.493 & 0.802 & 0.494 & 0.593 & 0.422 & 0.341 & 0.476 & 0.747 \\
$S_{\text{goal}}$ & 0.514 & 0.648 & 0.459 & 0.802 & 0.524 & 0.612 & 0.545 & 0.400 & 0.527 & 0.778 \\
$G_{\text{avg}}$ & 0.498 & 0.641 & 0.482 & 0.808 & 0.520 & 0.613 & 0.477 & 0.375 & 0.512 & 0.766 \\
$G_{\max}$ & 0.547 & 0.677 & \textbf{0.614} & \textbf{0.868} & 0.525 & 0.623 & 0.537 & 0.431 & 0.512 & 0.786 \\
\midrule
$\mathcal{C}_{\text{chain}}$ & 0.527 & 0.671 & 0.509 & 0.833 & 0.506 & 0.594 & 0.540 & 0.464 & 0.552 & 0.791 \\
\bottomrule
\end{tabular}
\end{adjustbox}
\caption{The strictly single-generation regime: AUROC and AURAC ($\uparrow$) when exactly one chain per question is scored by its own value (Gemini-generated answers, canonical test partition; no clustering or pool aggregation). Sampling-based methods do not exist in this regime. Avg is the unweighted mean of the four per-split values; bold marks the best value per column. The corresponding pooled-union values are reported in Appendix~\ref{app:overall}, where the $\mathcal{C}_{\text{chain}}$ row of this regime serves as the starkest example of the pooling bias: its pooled AUROC of 0.653 against near-chance per-split values.}
\label{tab:single-chain}
\end{table*}

Three findings follow. First, the coherence scores and $G_{\text{avg}}$ \emph{collapse to chance} (0.47--0.51 average AUROC): their discriminative power in the main protocol comes from the sum-share aggregation over the candidate pool, whose value is dominated by cluster size, i.e.\ by the agreement signal of the samples. They are therefore ensemble-level evidence, not properties of an individual chain that predict its correctness — which is consistent with, and motivates, their use as vote weights in Appendix~\ref{app:gwsc}. Second, $G_{\max}$ is the exception: it retains genuine single-chain signal (0.614 AUROC on Audio, where the candidate-pool protocol fails at 0.435) and attains the best average AUROC (0.547) and AURAC (0.677) among the geometric scores, so maximal step-to-input grounding is the one geometric quantity in our set that is informative about a chain in isolation. Third, the self-verbalisation baselines, which are single-chain by construction, dominate discrimination in this regime (Self-Probing 0.629 average AUROC and 0.715 average AURAC), at the cost of one additional call to the evaluated model. A related experiment in which each method \emph{selects} the answer purely by its own per-candidate score (a best-of-$n$ policy) degrades both accuracy and every UQ metric relative to majority voting for all methods, confirming the same reading: the geometric scores' value lies in modulating the ensemble, not in ranking candidates within a question.
